# Supplementary material for: LaForge: Always-Correct and Fast Incremental Builds from Simple Specifications
Source: arXiv:2108.12469 source file (2021-09-02)
Supplement: Supplementary file 1 [file appendix.tex]

\begin{appendices}

\section{State Types}
\label{appendix:state}

\riker's environment ($E$) models the UNIX filesystem and as a result, must contain analogues to all of the kinds of objects encountered in a real filesystem.
\riker also models ephemeral system state like pipes, sockets, and anonymous objects.
All of the above artifacts must be correctly modeled for builds to function as intended.
In this section, we describe the artifacts \riker models and how state is handled.

Note that all artifact types in \riker have \emph{metadata state}, represented by an \IRMetadataState object.
\texttt{uid}, \texttt{gid}, permissions, and artifact type are considered \IRMetadataState{}.
\riker considers all other attributes, like \texttt{mtime}, to be a part of an artifact's \emph{content state}.
\IRMetadataState{} is considered changed if any of its attributes are different.

\paragraph{Regular files.}
Regular files are represented in \riker's environment by a \FileArtifact data structure.
\FileArtifact{}s store both the last committed as well as uncommitted (i.e., model-only) \IRContentState.
\FileArtifact \IRContentState{}s can be cached, and if \riker caches it, it is written using its BLAKE3 hash as a filename to a three-level \file{cache} directory inside the \file{.rkr} directory.
\riker does not cache file contents that can be recreated on demand, like empty files.
A hash value and \texttt{mtime} is stored with a \IRContentState{}.
Content changes are always checked first by comparing \texttt{mtime}, and if they are different, by checking the \texttt{hash} value.
Uncommitted state takes precedence in a match over committed state.

\paragraph{Directories.}
\DirectoryArtifact{}s accurately model directory state, which is essential for obtaining correct behavior in cases like the motivating example (see~\sectref{sec:overview}) where files are incorporated into a build without changing the \rikerfile.
Like \FileArtifact{}s, they also keep committed and uncommitted state.
However, like UNIX directories, they also store references to other artifacts, including other \DirectoryArtifact{}s using a table that maps path strings to \DirectoryEntry{} objects.
The content of a \DirectoryArtifact{} is this table, and changes are determined by comparing all of the entries.
Like \FileArtifact{}s, uncommitted state takes precedence over committed state, but a \DirectoryEntry table may contain a mix of both committed and uncommitted state.
\riker can always commit directory contents on demand.

\paragraph{Pipes and Sockets.}
%Pipes have complicated semantics, and \riker models enough to be able to determine changes.
Unlike files and directories, \riker does not cache pipe state, which means that \riker's change logic for pipes is conservative, erring on the side of reporting changes.
Unlike files, pipe reads are side-effecting, and a read depends on the preceding read and any intervening writes.
When multiple commands write to the same pipe, this does not create dependencies between them.
For example, if \cmd{A} and \cmd{B} write to a pipe, and \cmd{C} reads that pipe, \cmd{C} transitively depends on \cmd{A} and \cmd{B} but neither \cmd{A} nor \cmd{B} depend on each other.
\riker therefore models reads and writes separately.
Since \riker does not cache pipe contents, if a command that reads a pipe needs to run, all readers and writers for the pipe need to run.
\riker currently models sockets as an uncacheable \FileArtifact{}, which is sufficient for change detection.

\paragraph{Symlinks.}
\SymlinkArtifact{}s store both committed and uncommitted content, and state is limited to storing a path.
Their relative simplicity means that they can be treated as if they are cached artifacts, and can be committed on demand.

\paragraph{Special files.}
Because ``everything is a file'' is a pervasive concept in UNIX, \riker finds dependencies on special files for all but the most trivial builds.
%A number of files, like \file{/dev/pts/0} and \file{/dev/urandom} represent hardware or other special devices.
%Some can be read and written, but others can only be read \emph{or} written.
\SpecialArtifact{}s allow \riker to specify change behavior on an \emph{ad hoc} basis.
At the start of each build, the \file{stdin} file descriptor refers to a \SpecialArtifact that is \emph{always changed};
% CC: Added the bit about the initial stdin fd because I don't want a reviewer to think we can't handle stdin/stdout redirection in Rikerfiles
the contents of \file{stdin} never match previously-observed state and cannot be committed, so any command that reads this file must rerun on every build.
Other special files like \file{/dev/tty}, \file{/dev/null}, and \file{/dev/urandom} are \emph{never changed};
reading or writing these files does not force a command to rerun.
% CC: Our definition of build equivalence allows us to treat any values read from /dev/urandom as acceptable.

\section{\traceir Language}
\label{appendix:traceir}

The \proc{Eval} function evaluates \traceir steps in the context of the given environment ($E$).
Whenever an \IRLaunch step is processed, and the target command is in the set of commands that must run ($R$), \proc{Eval} traces the command.
All other steps are emulated.

Here we describe the complete \traceir language.
We group steps according to whether they are concerned with artifact discovery, checking state, or updating state.
\traceir steps are generated by \riker's syscall layer from raw traces.

Command-related state like the starting directory, root directory, user, group, arguments, environment variables, and initial file descriptors are stored in the \IRCommand{} data structure.
Every step is associated with a given command.
The command at the root of the \traceir command tree is always \rkr.

\subsubsection*{Artifact Discovery Steps}
Although a build creates many artifacts (e.g., files), ultimately the operating system is responsible for creating and managing all state.
Consequently, there is little difference from \riker's standpoint between creating artifacts and discovering ones that already exist in the system.
Every access therefore refers to an existing artifact in the environment or creates a new one.
Each of the steps below creates an artifact in \riker's environment if it does not already exist, returning a \IRRef.
\IRRef{}s play a role akin to file descriptors.

\begin{lstlisting}[language=TraceIRSmall]
PathRef(cmd:|\IRCmdRef{}|, base:|\IRRef{}|,
        path:|\IRString{}|, flags:|\IRAccessFlags{}|): |\IRRef{}|
\end{lstlisting}
\vspace{-0.5em}
\noindent Returns a \IRRef whenever an artifact is accessed through a path.
Like UNIX paths, \texttt{PathRef} is relative to a base reference (like \IRCWD{}).
\texttt{PathRef} resolves to any type of artifact that can be accessed using a path.
\IRAccessFlags{} encodes the permissions required (read, write, execute) as well as other flags specific to the \syscall{open()} system call.

\begin{lstlisting}[language=TraceIRSmall]
FileRef(cmd:|\IRCmdRef{}|): |\IRRef{}| 
\end{lstlisting}
\vspace{-0.5em}
\noindent Returns a \IRRef{} to a new anonymous file.

\begin{lstlisting}[language=TraceIRSmall]
DirRef(cmd:|\IRCmdRef{}|): |\IRRef{}|
\end{lstlisting}
\vspace{-0.5em}
\noindent Returns a \IRRef{} to a new anonymous directory.

\begin{lstlisting}[language=TraceIRSmall]
PipeRef(cmd:|\IRCmdRef{}|): (|\IRRef{}|, |\IRRef{}|)
\end{lstlisting}
\vspace{-0.5em}
\noindent Returns \IRRef{}s to the read and write ends of a new anonymous pipe.

\begin{lstlisting}[language=TraceIRSmall]
SymlinkRef(cmd:|\IRCmdRef{}|, dest:|\IRString{}|): |\IRRef{}|
\end{lstlisting}
\vspace{-0.5em}
\noindent Returns a \IRRef{} to a new anonymous symbolic link with a given destination

\begin{lstlisting}[language=TraceIRSmall]
SpecialRef(cmd:|\IRCmdRef{}|): |\IRRef{}|
\end{lstlisting}
\vspace{-0.5em}
\noindent Returns a \IRRef{} to \file{stdin}, \file{stdout}, \file{stderr}, and the root directory (\file{/}).
This step provides a base \IRRef for artifact resolution, and is emitted statically in every trace.

\subsubsection*{State Check Steps.}
The following \traceir steps are emitted whenever a command reads from an artifact, and they record the state of the system during a trace.
State check steps are the primary means \riker has for detecting when changes occur, since a change will cause a state check to fail during emulation.
Note that artifact contents vary by artifact type and are described in~\sectref{sec:artifacts}.

\begin{lstlisting}[language=TraceIRSmall]
CompareRefs(cmd:|\IRCmdRef{}|, ref1: |\IRRef{}|,
            ref2: |\IRRef{}|, type: |\IRRefComparison{}|): |\IRBool{}|
\end{lstlisting}
\vspace{-0.5em}
\noindent
Compares two references.
When \texttt{type} is \IRSameInstance, the step returns \texttt{true} if \texttt{ref1} and \texttt{ref2} refer to the same artifact.
The converse is true when \texttt{type} is \IRDifferentInstance.

\begin{lstlisting}[language=TraceIRSmall]
ExpectResult(cmd:|\IRCmdRef{}|, ref: |\IRRef{}|,
             expected_result: |\IRInt{}|): |\IRBool{}|
\end{lstlisting}
\vspace{-0.5em}
\noindent
Checks that a reference, created using an artifact discovery step, \emph{resolves} to a given result.
Resolution in \riker models the \emph{path resolution algorithm} in Linux~\cite{pathresolution}. 
An expected result can either be \texttt{SUCCESS} when an artifact can be accessed through the given reference or a standard POSIX error code (e.g,. \texttt{ENOENT}).

\begin{lstlisting}[language=TraceIRSmall]
MatchMetadata(cmd:|\IRCmdRef{}|, ref: |\IRRef{}|, s: |\IRMetadataState{}|): |\IRBool{}|
\end{lstlisting}
\vspace{-0.5em}
\noindent
Checks that the referenced artifact is in the given metadata state \texttt{s}.

\begin{lstlisting}[language=TraceIRSmall]
MatchContent(cmd:|\IRCmdRef{}|, ref: |\IRRef{}|, s: |\IRContentState{}|): |\IRBool{}|
\end{lstlisting}
\vspace{-0.5em}
\noindent
Checks that the referenced artifact contains the given content state \texttt{s}.

\begin{lstlisting}[language=TraceIRSmall]
ExitResult(cmd:|\IRCmdRef{}|, child: |\IRCommand{}|,
           expected_code: |\IRInt{}|): |\IRBool{}|
\end{lstlisting}
\vspace{-0.5em}
\noindent
Checks that the exit code for the given child command has the given status.
During rebuild, this step also signals to the \riker runtime that the parent command must wait for the child to exit before proceeding.
This signal is important since a parent might be emulated while its child is traced.

\subsubsection*{State Update Steps}
The following \traceir steps are emitted whenever a command alters system state, and they record precisely how state is updated.
During emulation, these steps alter environment state.
Like state checks, they can also signal a change if their operations yield different results.

\begin{lstlisting}[language=TraceIRSmall]
UpdateMetadata(cmd:|\IRCmdRef{}|, ref: |\IRRef{}|, s: |\IRMetadataState{}|): |\IRBool{}|
\end{lstlisting}
\vspace{-0.5em}
\noindent
Updates the referenced artifact's metadata with the given state.

\begin{lstlisting}[language=TraceIRSmall]
UpdateContent(cmd:|\IRCmdRef{}|, ref: |\IRRef{}|, s: |\IRContentState{}|): |\IRBool{}|
\end{lstlisting}
\vspace{-0.5em}
\noindent
Updates the referenced artifact's content with the given state.

\begin{lstlisting}[language=TraceIRSmall]
AddEntry(dir: |\IRRef{}|, name: |\IRString{}|, target: |\IRRef{}|): |\IRBool{}|
\end{lstlisting}
\vspace{-0.5em}
\noindent
Adds an entry to the referenced directory with the given name and target artifact.

\begin{lstlisting}[language=TraceIRSmall]
RemoveEntry(dir: |\IRRef{}|, name: |\IRString{}|, target: |\IRRef{}|): |\IRBool{}|
\end{lstlisting}
\vspace{-0.5em}
\noindent
Removes the entry with the given name and target artifact from the referenced directory.

\begin{lstlisting}[language=TraceIRSmall]
Launch(cmd:|\IRCmdRef{}|, child: |\IRCommand{}|): |\IRCmdRef{}|
\end{lstlisting}
\vspace{-0.5em}
\noindent
Models the launch of a child command.

\begin{lstlisting}[language=TraceIRSmall]
UsingRef(cmd:|\IRCmdRef{}|, ref: |\IRRef{}|)
\end{lstlisting}
\vspace{-0.5em}
\noindent
Signals the start of the lifetime of a \IRRef{}.
This step is needed for references that are shared between commands and whose lifetime needs to be controlled so that references can be correctly disposed.
For example, pipes are shared and must be closed otherwise commands that use them with blocking semantics will hang.
By default, \IRRef{} lifetime is assumed to be linked to command lifetime.

\begin{lstlisting}[language=TraceIRSmall]
DoneWithRef(cmd:|\IRCmdRef{}|, ref: |\IRRef{}|)
\end{lstlisting}
\vspace{-0.5em}
\noindent
Signals the end of a reference lifetime.

\begin{lstlisting}[language=TraceIRSmall]
Exit(cmd:|\IRCmdRef{}|, code: |\IRInt{}|)
\end{lstlisting}
\vspace{-0.5em}
\noindent
Records that the given command exits with the given code.

\section{Incorrect Redis \Makefile}
\label{appendix:redis}

Redis comes with a \Makefile that generates a \file{version.h} header using the current \cmd{git} hash.
The following is the relevant excerpt (line breaks added).

\begin{verbatim}
GIT_SHA1=`(git show-ref --head --hash=8 \
  2> /dev/null || echo 00000000) | head -n1`
GIT_DIRTY=`git diff --no-ext-diff \
  2> /dev/null | wc -l`
BUILD_ID=`uname -n`"-"`date +%s`
echo "#define REDIS_GIT_SHA1 \"$GIT_SHA1\"" \
  > release.h
echo "#define REDIS_GIT_DIRTY \"$GIT_DIRTY\"" \
  >> release.h
echo "#define REDIS_BUILD_ID \"$BUILD_ID\"" \
  >> release.h	
\end{verbatim}

Unfortunately, \file{version.h} is not updated with the correct \texttt{REDIS\_GIT\_DIRTY} variable when code in the repository is modified.
While \make can indeed include arbitrary embedded shell code, the Redis \Makefile does not actually encode a dependence for \file{version.h} on the output of \cmd{git}.
Encoding this dependence in \make is nontrivial.
\riker has no such limitation, inferring the dependence automatically and correctly.

\end{appendices}
